# Supplementary material for: Text-Guided Image Clustering
Source: arXiv:2402.02996 source file (2024-02-19)
Supplement: Supplementary file 1 [file caption.tex]

% \begin{figure}[htb]
% \centering
% \includegraphics[width=\columnwidth]{aux/plots/appendix_num_captions_full.pdf}
% \caption{Investigation, how many captions should be sampled per image. Number of Captions is on x-axis, mean and standard deviation of clustering performance is on y-axis.}
% \label{fig:appendix_num_captions}
% \end{figure}
