# Supplementary material for: Text-Guided Image Clustering
Source: arXiv:2402.02996 source file (2024-02-19)
Supplement: Supplementary file 2 [file keywords_vqa.tex]

\section{Keyword-Guided Clustering}

\begin{figure*}
     \centering
     \begin{subfigure}[b]{0.48\textwidth}
         \centering
         \includegraphics[width=\textwidth]{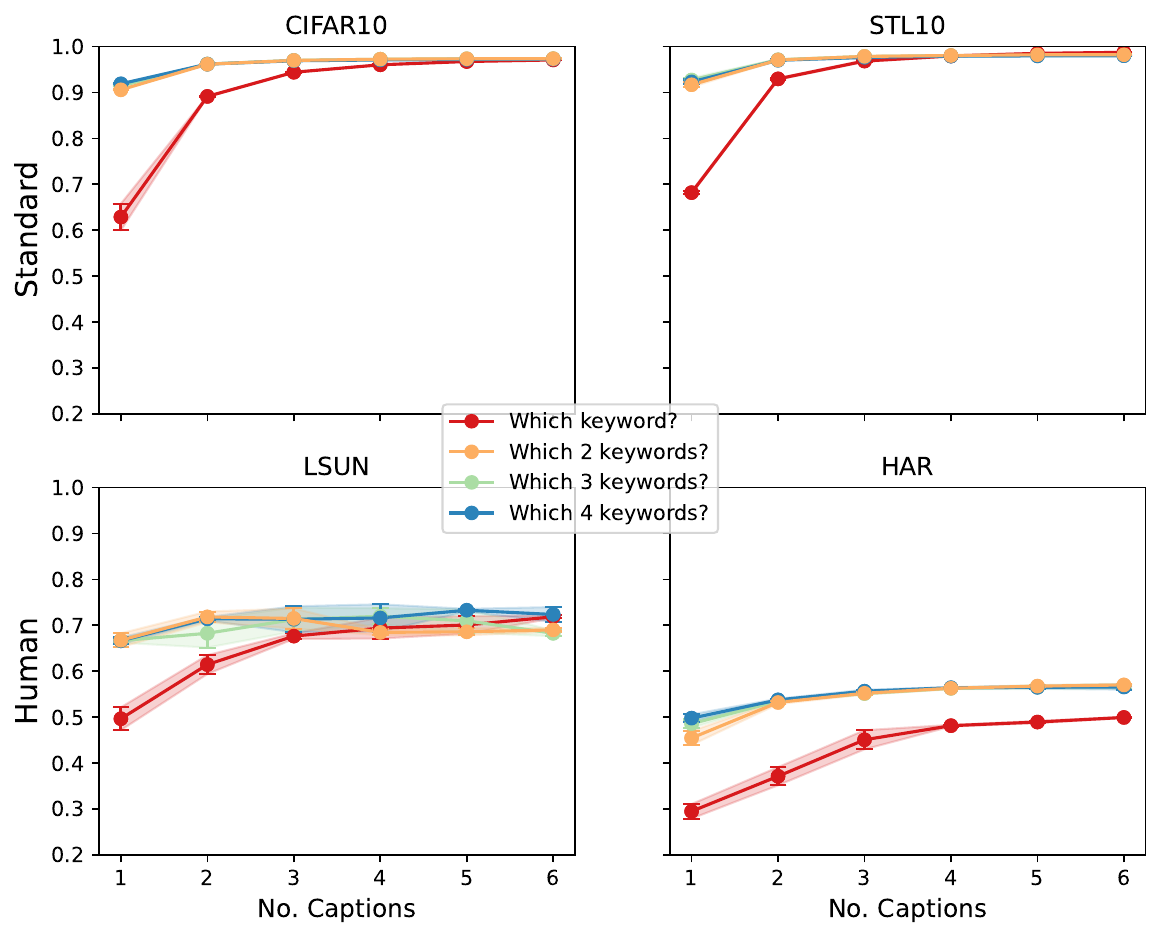}
         \caption{SBERT Acc}
         \label{fig:appdx_num_kws_sbert_acc}
     \end{subfigure}
     \hfill
     \begin{subfigure}[b]{0.48\textwidth}
         \centering
         \includegraphics[width=\textwidth]{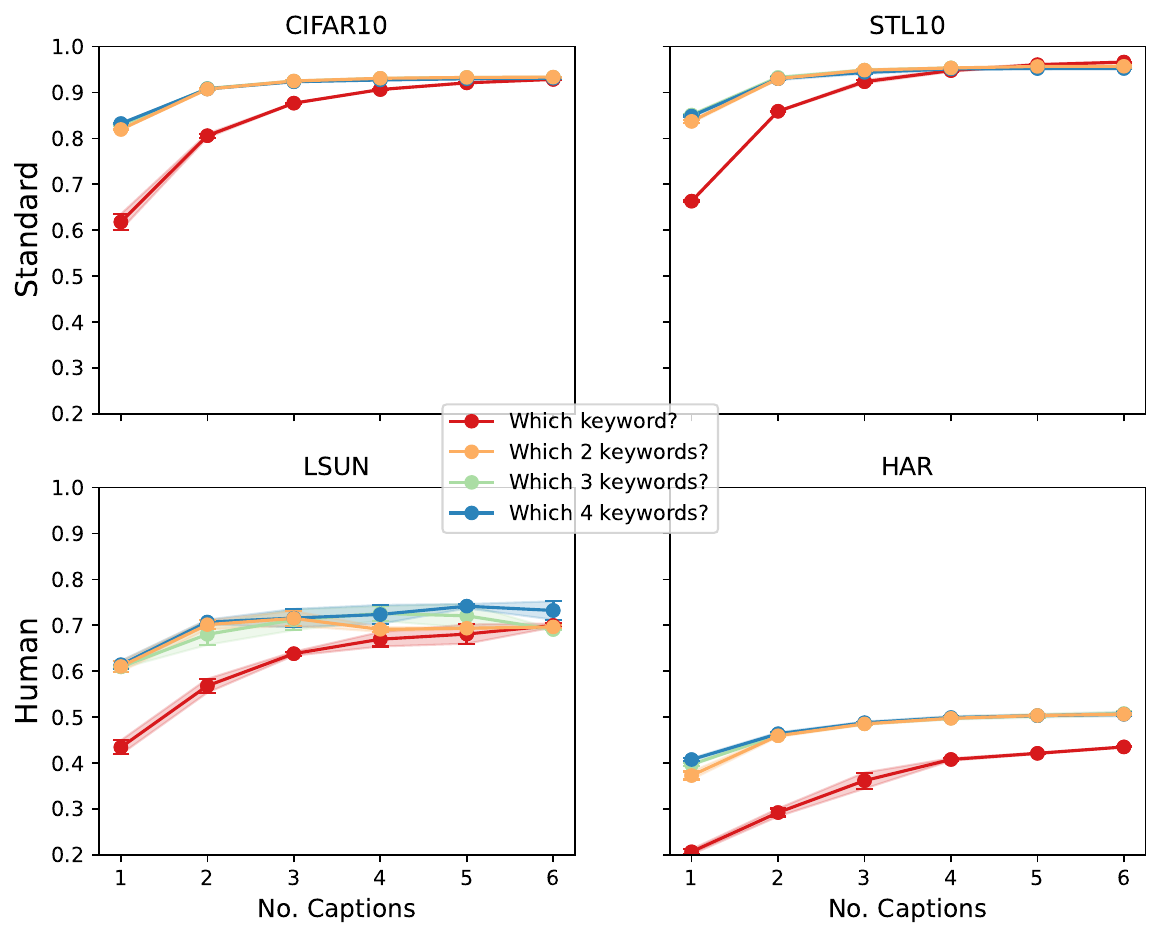}
         \caption{SBERT NMI}
         \label{fig:appdx_num_kws_sbert_nmi}
     \end{subfigure}
     \hfill
     \begin{subfigure}[b]{0.48\textwidth}
         \centering
         \includegraphics[width=\textwidth]{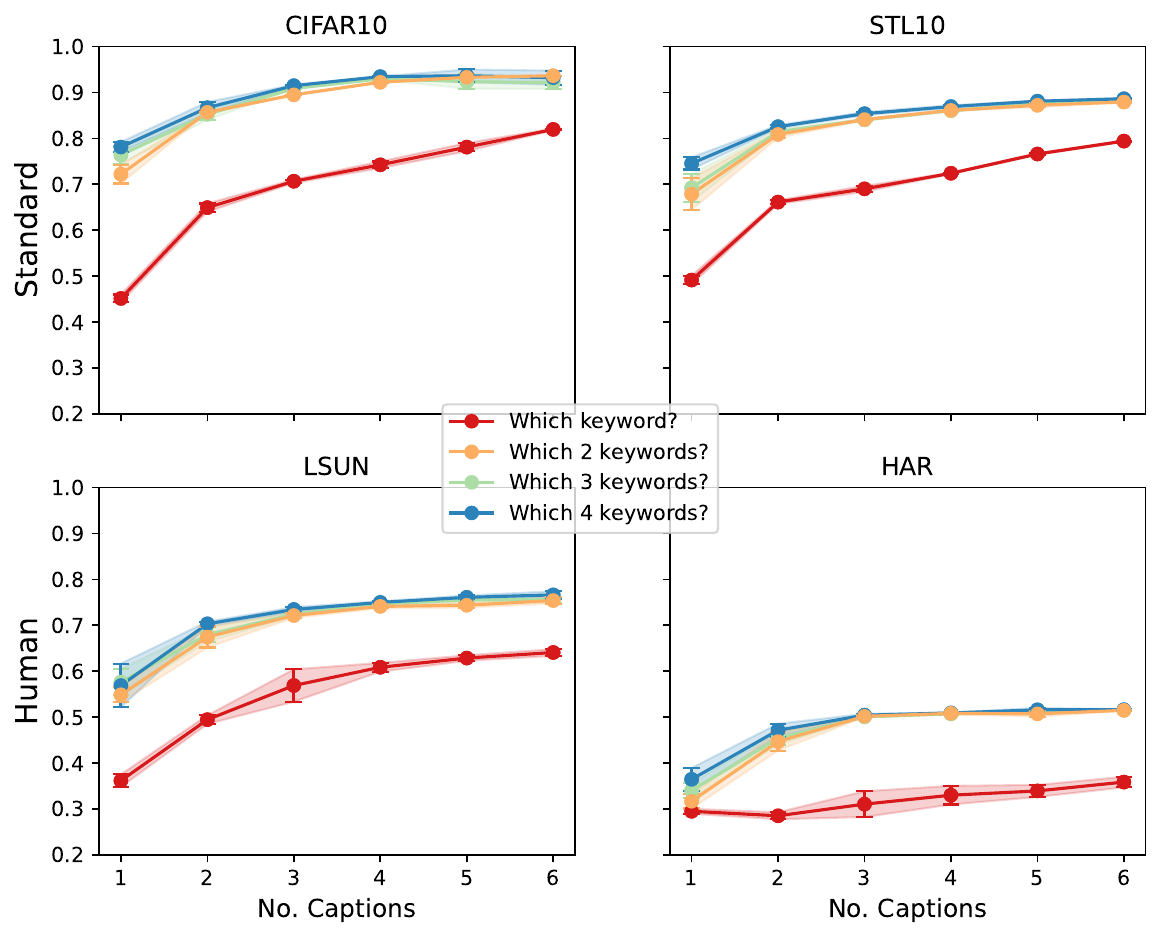}
         \caption{TF-IDF Acc}
         \label{fig:appdx_num_kws_tfidf_acc}
     \end{subfigure}
     \begin{subfigure}[b]{0.48\textwidth}
         \centering
         \includegraphics[width=\textwidth]{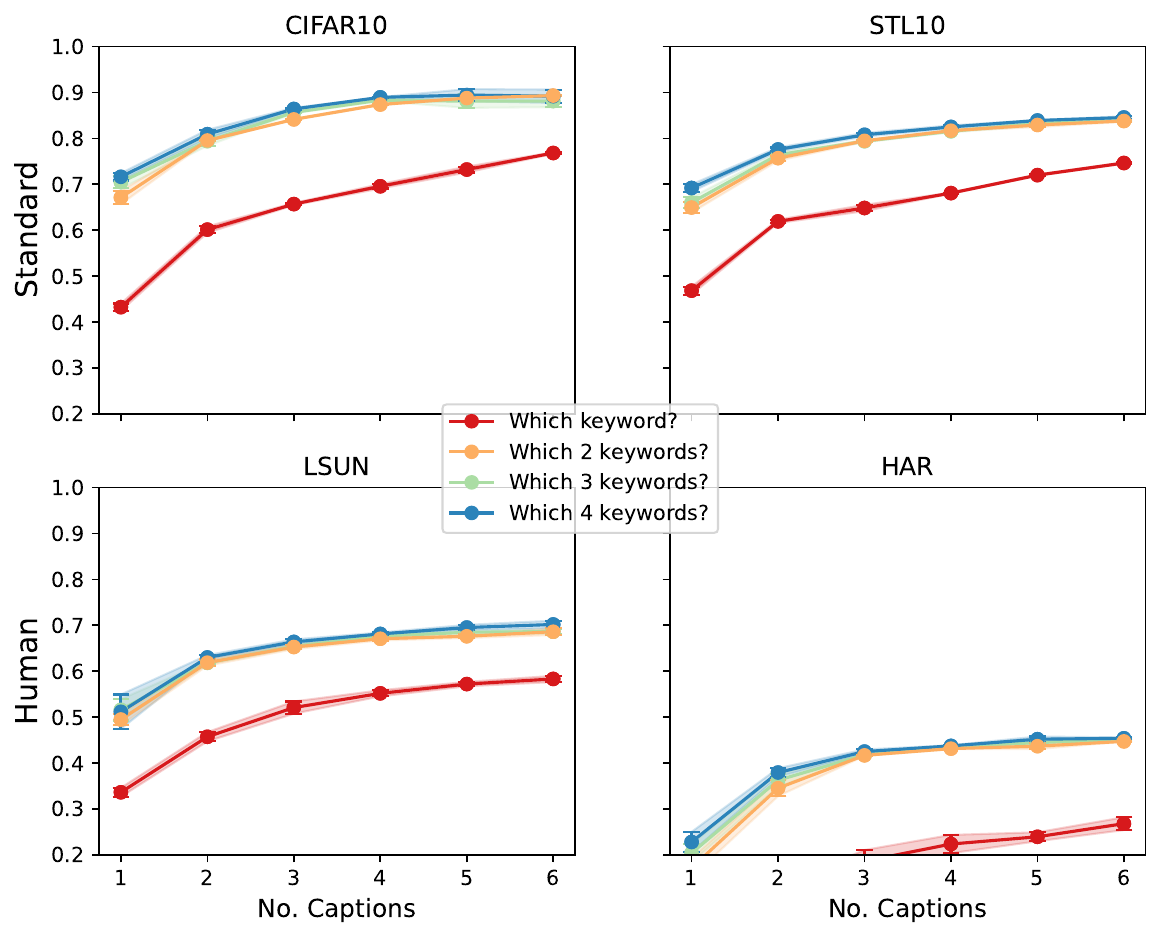}
         \caption{TF-IDF NMI}
         \label{fig:five over x}
     \end{subfigure}
        \caption{Three simple graphs}
        \label{fig:appdx_num_kws_tfidf_nmi}
\end{figure*}
